# Supplementary material for: Deep-STORM: super-resolution single-molecule microscopy by deep learning
Source: arXiv:1801.09631 ancillary file (2018-05-02)
Supplement: Supplementary file 1 [file supplementary.pdf]

# Deep-STORM: supplementary material

Elias Nehme[1,2,*], Lucien E. Weiss[2], Tomer Michaeli[1], and Yoav Shechtman[2]

[1]Department of Electrical Engineering, Technion, 32000 Haifa, Israel
[2]Department of Biomedical Engineering, Technion, 32000 Haifa, Israel
[*]Corresponding author: seliasne@campus.technion.ac.il

## 1 Neural network architecture details

The proposed network architecture is depicted in Fig. 1. The architecture is composed of 4 different types of blocks, each highlighted in a different color for distinction. A hierarchy of feature representations with a varying numebr of channels is obtained through successive convolutions and pooling layers. The spatial supports of all the convolutional filters are $3 \times 3$. Each convolution layer is followed by a Batch Normalization (BN) layer [1], and an element-wise ReLU non-linearity [2]. The number of features in the representation is increased from 32 up to 512, and then reduced back to 32 for the final pixel-wise prediction step. Let $x$ be the input grayscale image, and $f_k$ be the $k^{th}$ out of $N$ convolutional filters, the $k^{th}$ output feature map of a convolution layer is given by

$$y_k = f_k \circledast x, \tag{1}$$

where $\circledast$ denote 2D convolution. Let $\mu^{\mathcal{B}}$ and $\sigma^{\mathcal{B}}$ denote the empirical mean and standard deviation of the feature maps over a mini-batch $\mathcal{B} = \{x_1, ..., x_M\}$, where $M$ refers to the number of samples in the mini-batch. Let $\beta_k$ and $\gamma_k$ be the learned mean and standard deviation for the $k^{th}$ feature map, the $k^{th}$ output of the BN layer is given by

$$z_k = \gamma_k \times \frac{y_k - \mu_k^{\mathcal{B}}}{\sigma_k^{\mathcal{B}}} + \beta_k, \tag{2}$$

The final feature representation is given by $o_k = ReLU\,(z_k) = \max\,(z_k, 0)$. The width of each block (Fig. 1) is proportional to the number of channels in the representation.
Max-Pooling ($2 \times 2$) refers to a spatial down-sampling operation [3], acting on each feature map in the input volume separately. For each input feature map of size $K \times K$, the output of the Max-Pooling ($2 \times 2$) block is a feature map of size $\frac{K}{2} \times \frac{K}{2}$, where each element corresponds to the maximal value in the matching distinct $2 \times 2$ region in the input feature map.
Up-sampling ($2 \times 2$) refers to a spatial up-sampling operation, acting on each feature map in the input volume separately. For each input feature map of size $K \times K$, the output of the Up-sampling ($2 \times 2$) block is a feature map of size $2K \times 2K$, where each element is replicated to a $2 \times 2$ region, to recover the spatial span. Finally, the Conv ($1 \times 1$) block outputs a single image, which is a weighted sum of the channels of it's input.

## 2 Training data preparation

We demonstrated training on both simulated and experimental examples. In each case, the training dataset was prepared slightly differently as a result of the number of available examples.

### 2.1 Simulated training examples

For the generation of simulated training examples, we used the ImageJ [4, 5] ThunderSTORM [6] plugin. The parameters for the simulated data generator were approximately matched to the experimental data to be evaluated. Specifically, for a given imaging setup, the camera specifications included setting the pixel size [nm], photo-electrons per A/D count, quantum efficiency, base level [A/D] counts, and the EM gain for an EMCCD camera, or the readout noise $\left[\frac{electrons}{pixel}\right]$ for a CMOS camera. The experimental sample parameters included setting the PSF model (e.g. Integrated Gaussian), the range of FWHM of the PSF [nm], intensity range of the emitters [photons], expected density $\left[\frac{emitters}{\mu m^2}\right]$, and the mean background photons per pixel [photons]. In case of a linear drift, the drift distance [nm] and the drift angle [deg.] could be also incorporated into the simulation, to train a more precise and unbiased estimator.
For each experiment, we matched the experimental parameters, and simulated twenty $64 \times 64$ images with randomly positioned emitters. Afterwards, the simulated images and the list of simulated positions were loaded in MATLAB. From each simulated image we extracted 500 random $26 \times 26$ regions, and their respective ground truth $xy$ positions. Next, each region was up-sampled by a factor of 8 using a simple nearest-neighbor interpolation, and the appropriate positions were projected on the high-resolution grid, yielding an image with spikes. The result is a set of 10K pairs of upsampled low-resolution regions ($208 \times 28$ pixels), alongside images with spikes at the ground truth positions used as training examples. The 10K regions were split into a 7K training set, and 3K validation set to prevent over-fitting.

### 2.2 Experimental training examples

For the generation of experimental training examples, we acquired a dataset of 100 sparse frames of quantum dots. Next, the emitters in each frame were localized using ThunderSTORM in single-emitter fitting mode. We did not acquire dense frames, to ensure the emitters' ground truth positions could be recovered with high-precision. The resulting list of positions and the acquired experimental images were loaded in MATLAB, to be divided into two distinct datasets - for training and for testing. To ensure only reasonably bright emitters are incorporated in both the training and testing phases, emitters with an intensity below 1000 photons were excluded from the experimental images, and replaced with random noise. From each experimental image ($1200 \times 1200$, with a pixel size of 110 nm), we extracted all distinct $26 \times 26$ regions that contained at least a single emitter, accompanied by the localized positions obtained from Thunder-

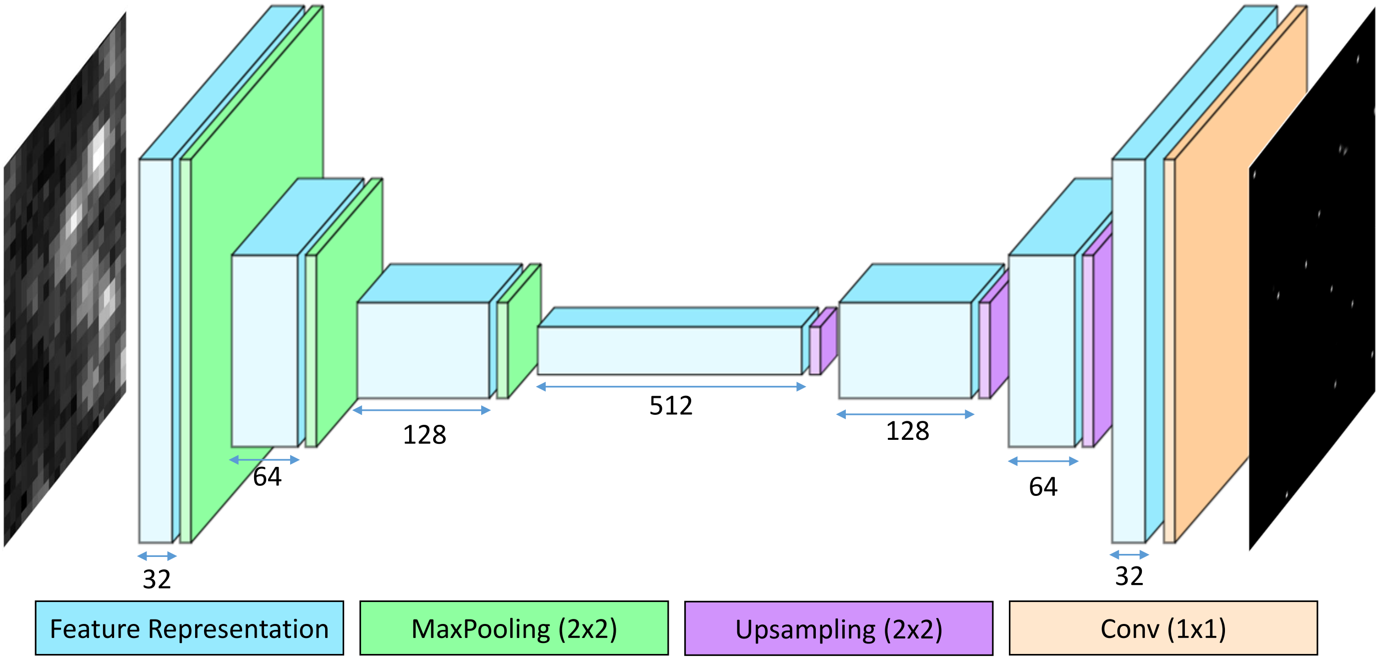


**Fig. 1.** Fully convolutional architecture details. The number below each Conv ($3 \times 3$)-BN-ReLU block refers to the number of convolutional filters in the respective convolutional layer.

STORM. The result was 1560 distinct regions, without overlaps, to avoid contamination of the training set. The regions were split into 1200 regions for training, and 360 regions for testing. To generate a challenging higher density datasets, we combined 8 randomly chosen regions at a time. To diversify the combinations, each region was first randomly rotated by an angle $\theta \in \{0^0, 90^0, 180^0, 270^0\}$. Similarly to the simulated examples, the combined regions were upsampled by a factor of 8 using nearest neighbor interpolation, and accompanied by images containing spikes at the respective ground truth positions. The result was a training set composed of 10K combinations of 1200 regions, and a test set composed of 3K combinations of ***different*** 360 regions.

### 2.3 Normalization

To ensure invariance of the learned estimator to the absolute photon counts of emitters intensity and background, we scale each upsampled region intensity to the range $[0, 1]$. The final examples are normalized by the mean and averaged standard deviation (per-upsampled region) of the dataset without additional data augmentation.

## 3 Precision evaluation

To evaluate the precision of Deep-STORM, in a context similar to localization microscopy, we simulated a blinking movie of dense emitters positioned along a line with a width of 1 nm (red, Fig. 2 (a)), and measured the FWHM of a Gaussian fitted to the effective PSF ( Fig. 2). The simulation pixel size was 100 nm, the PSF model was Integrated-Gaussian with a FWHM of $\sim 350\ nm$, the density was 3 $\left[\frac{emitters}{\mu m^2}\right]$, and the intensity of the emitters was 1000 photons with a mean background of 10 $\left[\frac{photons}{pixel}\right]$, with no additional readout noise. The resulting FWHM of Deep-STORM on a $12.5\ nm$ grid was $24\ nm$ (black triangles, Fig. 2 (b)), $\sim 14\times$ smaller than the size of the diffraction-limited PSF.

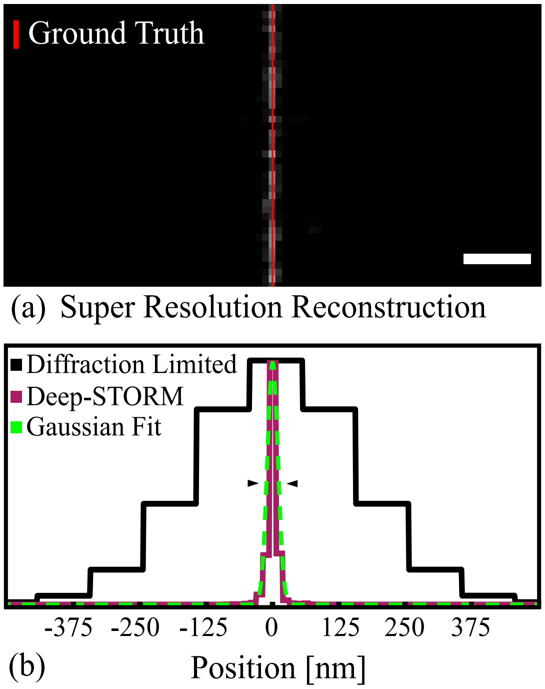


**Fig. 2.** Quantification of precision. (a) Deep-STORM recovery with the ground truth (red) super-imposed. (b) Reconstruction summed along the linear axis (magenta), and fit with a Gaussian (green) to estimate the precision. The FWHM (black triangles) was 24 nm.

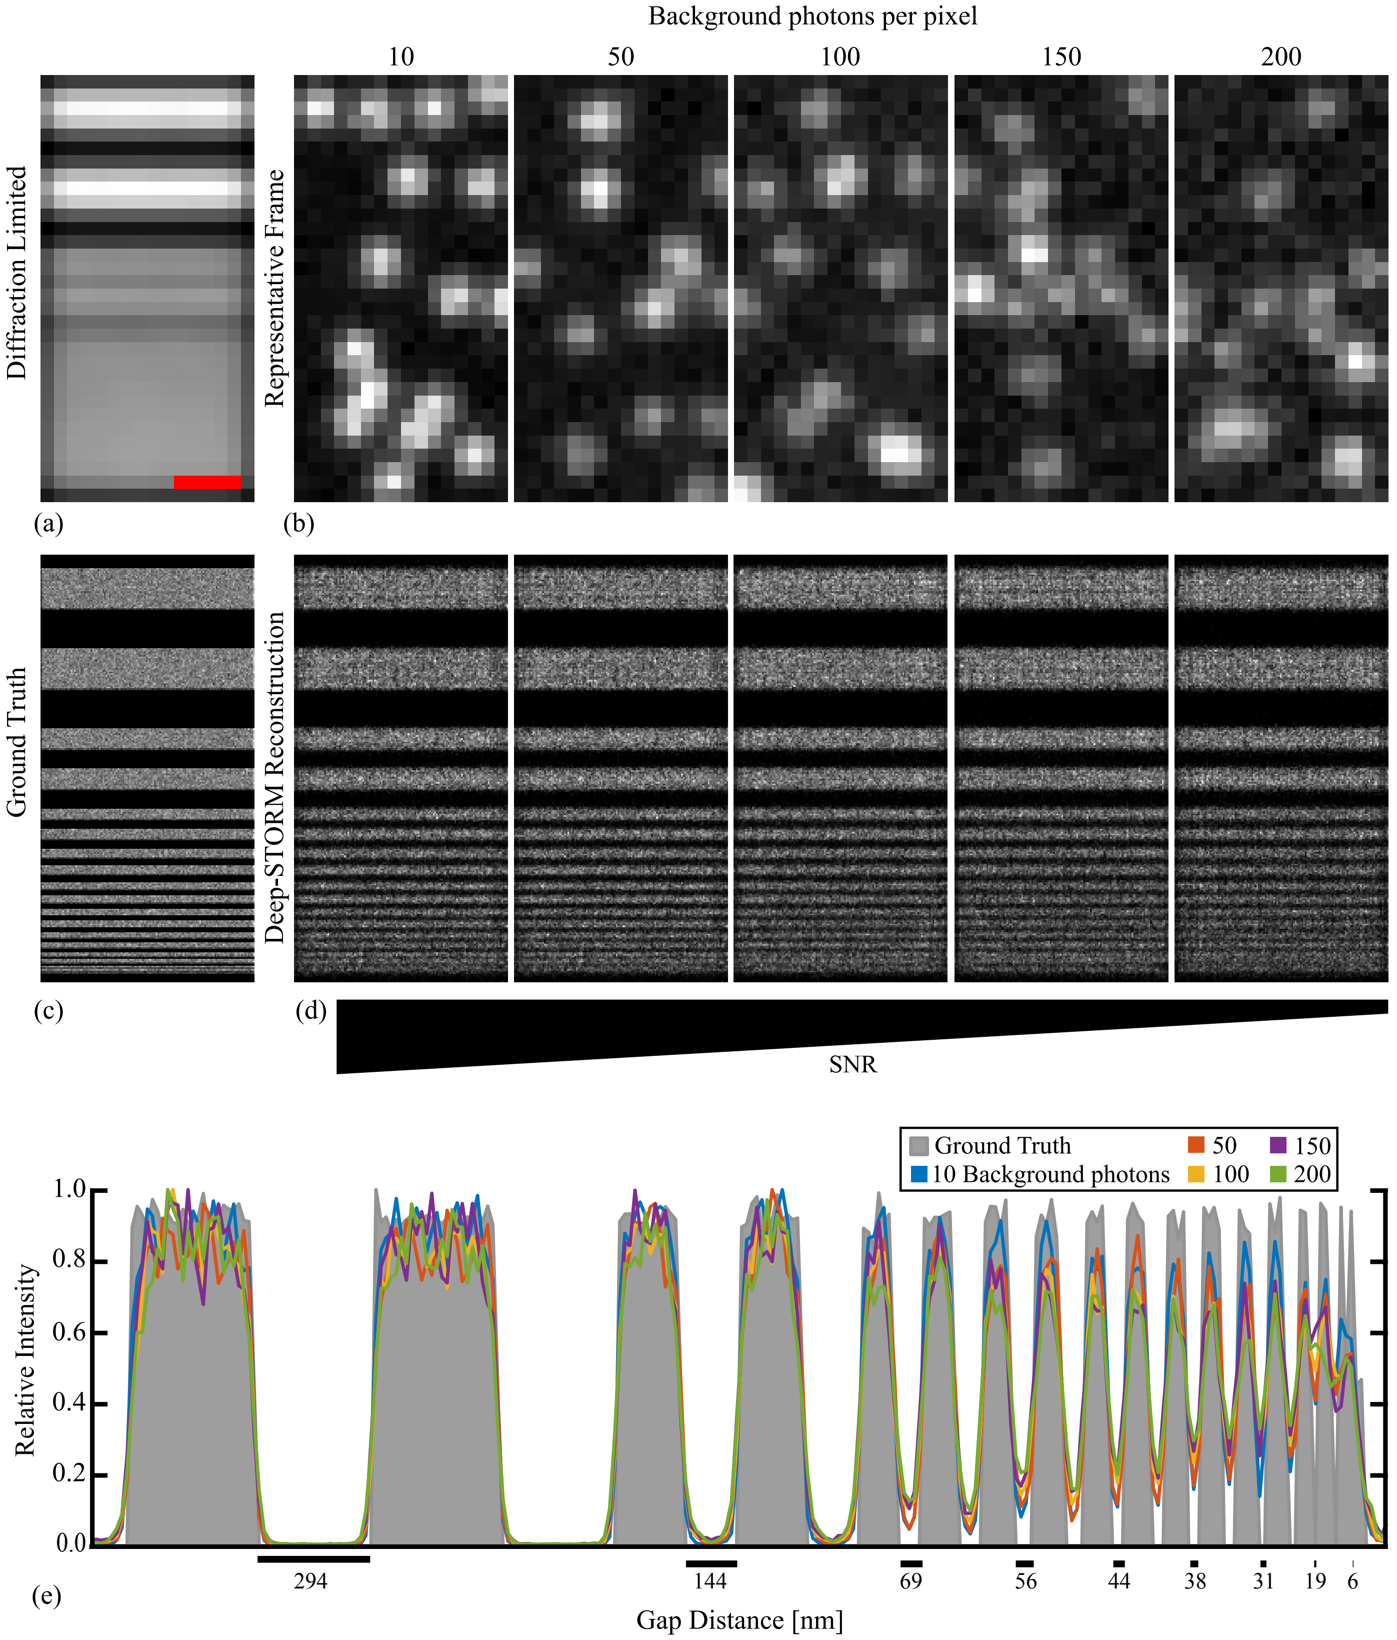


**Fig. 3.** Resolution and signal-to-noise. (a) Diffraction-limited image of horizontal lines, scale bar 500 nm. (b) Simulated single-frames of emitters with various numbers of background photons per pixel, 1000 signal photons per emitter, and a density of 3 emitters per square micron. (c) The ground truth positions of simulated emitters. (d) Deep-STORM reconstructed images. (e) Sum along the horizontal axis of the reconstruction intensities.

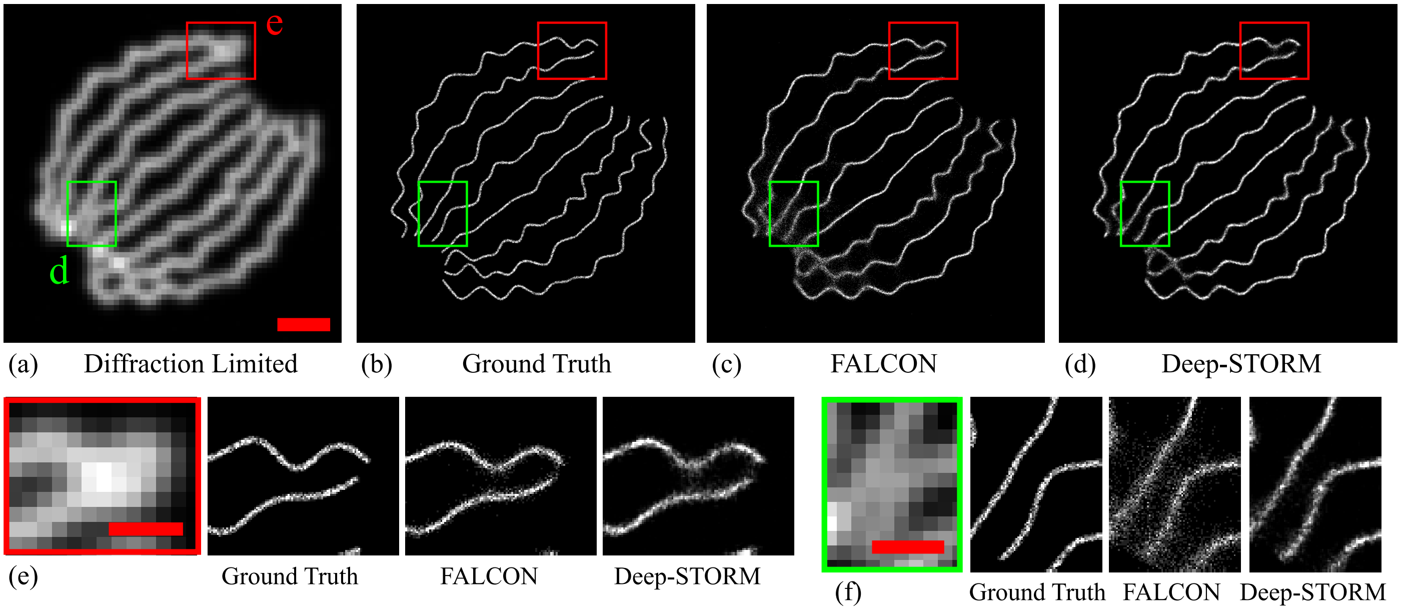


**Fig. 4.** Simulated microtubules (Comparison to FALCON). (a) Sum of the acquisition stack. Scale bar is 1 $\mu m$. (b) Ground truth. (c) Reconstruction by FALCON (d) Reconstruction by Deep-STORM. (e)-(f) Magnified views of two selected regions. Scale bars are 0.5 $\mu m$.

## 4 Resolution quantification

We quantified the resolution of Deep-STORM for different density (Fig. 3 main text) and SNR (Fig. 3) conditions, by recovering simulated blinking emitters along a grid of horizontal stripe pairs, with a gradually decreasing gap distance. The simulation pixel size was 100 nm. The PSF model was Integrated-Gaussian with a FWHM of $\sim$ 275 nm. The density was 3 $\left[\frac{emitters}{\mu m^2}\right]$, and the intensity of the emitters was 1000 photons with a varying mean background of $\{10, 50, 100, 150, 200\}$ $\left[\frac{photons}{pixel}\right]$, and no additional readout noise. For a low background of 10 $\left[\frac{photons}{pixel}\right]$, Deep-STORM was able to resolve lines with a 19 nm gap showing a resolution close to the recovery pixel size (12.5 nm). In addition, for a very high background of 200 $\left[\frac{photons}{pixel}\right]$, Deep-STORM was able to achieve a resolution of at least 31 nm.

## 5 Comparison to FALCON

We tested Deep-STORM on super-resolution data, and benchmarked against the fast multi-emitter fitting algorithm FALCON [7]. First, we reconstructed a simulated microtubule dataset available on the EPFL SMLM challenge website [8] (Fig. 4).

The optimal parameters for FALCON were set empirically through a comprehensive trial and error process, such that spurious detections are minimized, and the number of recovered positions was roughly equal to the number of underlying emitters. The resulting values were: wavelet decomposition level of 6, threshold level of $T = 0.05$, $\delta T = 1.1$, sparsity of 2, upsampling factor for deconvolution of 8, upsampling factor for refinement of 8, 500 iterations for step 1, 140 iterations for step 2, 20 iterations for step 3, 100 background iterations for step 1, 70 background iterations for step 2, 300 iterations for background standard deviation $\sigma$, and $\delta\sigma = 0.15$.

Since Deep-STORM is not constrained to output emitter positions, we quantified the quality of the results based on image similarity measures, rather than a point-list comparison (e.g. Jaccard index). Specifically, we used the standard normalized mean square error: $NMSE(\hat{x}, x) = \frac{\|\hat{x}-x\|_2^2}{\|x\|_2^2} \times 100\%$. Deep-STORM showed improved NMSE of 37% compared to 61% for FALCON. Deep-STORM managed to resolve nearby microtubule edges (Fig. 4) and recovered the underlying structure curvature slightly more accurately compared to FALCON (highlighted in white arrows in Fig. 5).

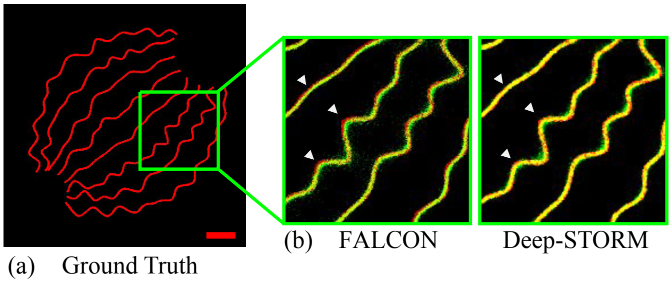


**Fig. 5.** Reconstruction accuracy (Comparison to FALCON). (a) Ground truth image of simulated microtubules. Scale bar is 1 $\mu$m. (b) Merged reconstruction with the ground truth. Red shows the ground truth, green corresponds to the recovery result, and yellow marks their overlap. Note that FALCON (left) does not follow the twisted shape in all places (white triangles), while Deep-STORM (right) better recovers the underlying structure.

Second, we tested the result of Deep-STORM on experimental data obtained from Sage et al. [8], training solely on simulated data with similar experimental conditions - namely, SNR and emitter density. Deep-STORM recovery is more precise with less spurious localizations occluding fine structures (Fig. 6).

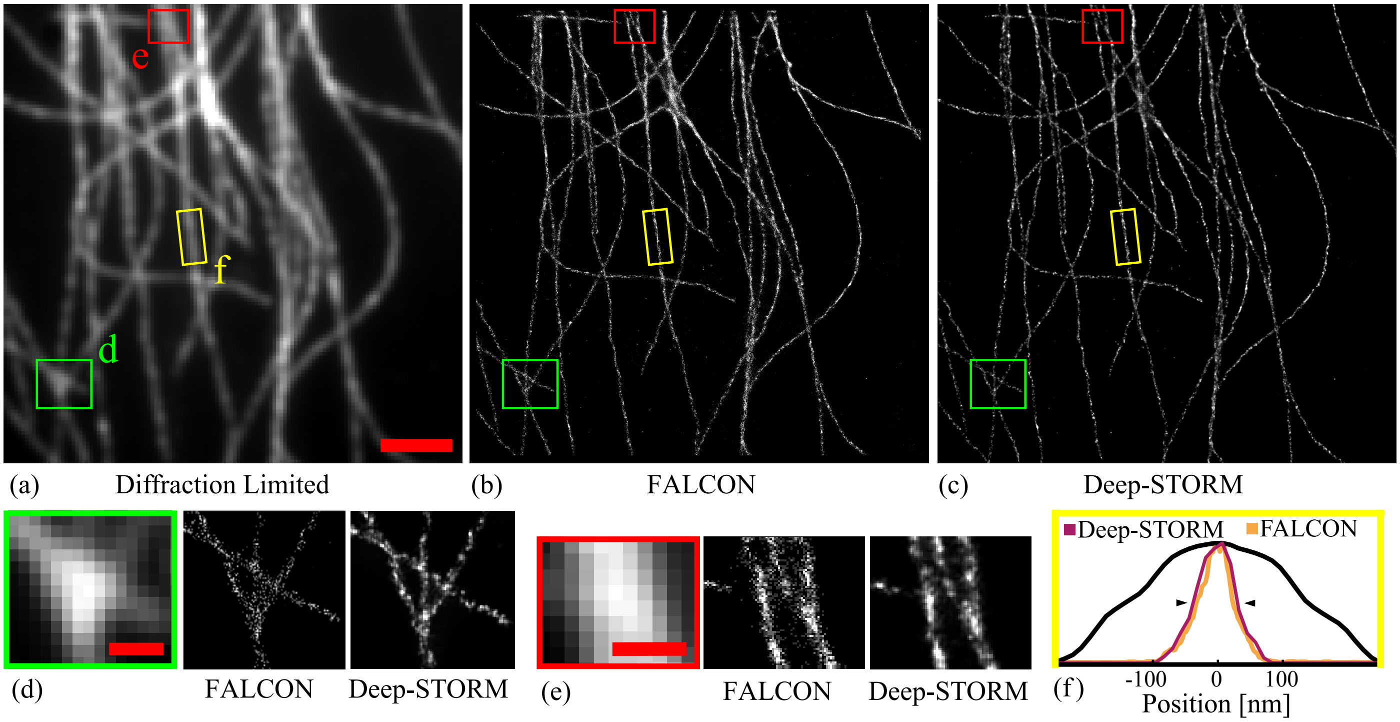


**Fig. 6.** Experimentally measured microtubules (Comparison to FALCON). (a) Sum of the acquisition stack. Scale bar is 2 $\mu m$. (b) Reconstruction by the FALCON. (c) Reconstruction by Deep-STORM. (d)-(e) Magnified views of two selected regions. Scale bars are 0.5 $\mu m$. (f) The width projection of the highlighted yellow region. The attained FWHM (black triangles) for FALCON was 54 $nm$ and 67 $nm$ for Deep-STORM. The black line shows the diffraction-limited projection.

## 6 Training on simulated vs. experimental data

To test the effect of training on simulated as opposed to experimental examples, we trained and tested Deep-STORM on an experimental QD dataset. The training examples were prepared as explained in section 2. The resulting imaging conditions were challenging: The emitter density of the regions was around $2\left[\frac{emitter}{\mu m^2}\right]$, there were $\sim 2500$ mean signal photons per emitter, and a total additive Gaussian noise with a standard deviation of 20 photons. To quantify the results, we counted the total number of emitters detected by both nets using a threshold of 1, where each connected blob of pixels was counted as one emitter. True positives refer to emitters predicted within a radius of 70 nm from a ground truth position. False positives refer to the remaining predicted blobs. Reconstruction using a net trained on experimental data resulted in 96% true positive rate with only 1.6% false positive rate, compared to 87.8% true positive rate with 8.7% false positive rate when reconstructing the same data using a net trained on simulatd examples (Fig. 7). Note that, because of the low number of different emitters present in the experimental training set, the network tends to predict wider "blobs" as opposed to 1-2 pixel predictions by the network trained on simulated examples, with a more rich and diverse training set. This could be mitigated by acquiring a larger number of experimental frames, or alternatively acquiring denser frames and using a more sophisticated data post-processing method accompanied by an improved multi-emitter fitting algorithm.

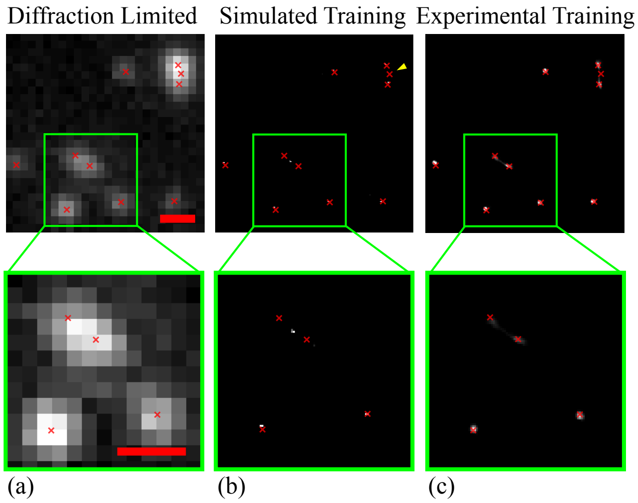


**Fig. 7.** Simulated versus experimental training on QD data. (a) Diffraction limited image of dense fields of QDs created from sums of 8 sparse regions. Red crosses show the underlying positions determined by Thunderstorm in sparse images. (b) Deep-STORM reconstruction using a simulated training set of overlapping Gaussians with a similar density, signal and background. Yellow arrow highlights an unrecovered emitter. (c) Deep-STORM reconstruction using an equivalent dataset formed from experimental images. Scalebars are 500 nm.

# 7 Robustness

We tested the robustness of Deep-STORM to a density mismatch between the training data and the measured dataset, by evaluating the reconstruction of a *high* density dataset with networks trained for *lower* densities. In addition, we also evaluated the reconstruction of a *low* density dataset with networks trained for *higher* densities (Fig. 8). A similar analysis was performed for SNR mismatch between the training data and the measured dataset (Fig. 9). Deep-STORM proved to be relatively robust to a $\sim 2 \left[\frac{emitters}{\mu m^2}\right]$ density mismatch (Fig. 8 (e-f)). Moreover, in case of SNR uncertainity and enough blinking data, we found it preferable to train a net on an under-estimation of the background photons (Fig. 9 (c)), rather than to overshoot (Fig. 9 (d)), thereby preventing a high false positive rate.

# References


[1] S. Ioffe and C. Szegedy, "Batch normalization: Accelerating deep network training by reducing internal covariate shift," in *Proceedings of the 32nd International Conference on Machine Learning* (F. Bach and D. Blei, eds.), vol. 37 of *Proceedings of Machine Learning Research*, (Lille, France), pp. 448–456, PMLR, 07–09 Jul 2015.

[2] A. L. Maas, A. Y. Hannun, and A. Y. Ng, "Rectifier Nonlinearities Improve Neural Network Acoustic Models," *Proceedings of the 30 th International Conference on Machine Learning*, vol. 28, p. 6, 2013.

[3] D. Scherer, A. Müller, and S. Behnke, "Evaluation of pooling operations in convolutional architectures for object recognition," *Lecture Notes in Computer Science (including subseries Lecture Notes in Artificial Intelligence and Lecture Notes in Bioinformatics)*, vol. 6354 LNCS, no. PART 3, pp. 92–101, 2010.

[4] C. T. Rueden, J. Schindelin, M. C. Hiner, B. E. DeZonia, A. E. Walter, E. T. Arena, and K. W. Eliceiri, "Imagej2: Imagej for the next generation of scientific image data," *BMC Bioinformatics*, vol. 18, p. 529, Nov 2017.

[5] J. Schindelin, I. Arganda-Carreras, E. Frise, V. Kaynig, M. Longair, T. Pietzsch, S. Preibisch, C. Rueden, S. Saalfeld, B. Schmid, J.-Y. Tinevez, D. J. White, V. Hartenstein, K. Eliceiri, P. Tomancak, and A. Cardona, "Fiji: an open-source platform for biological-image analysis," *Nature Methods*, vol. 9, pp. 676–682, jun 2012.

[6] M. Ovesný, P. Křížek, J. Borkovec, Z. Švindrych, and G. M. Hagen, "ThunderSTORM: A comprehensive ImageJ plug-in for PALM and STORM data analysis and super-resolution imaging," *Bioinformatics*, vol. 30, no. 16, pp. 2389–2390, 2014.

[7] J. Min, C. Vonesch, H. Kirshner, L. Carlini, N. Olivier, S. Holden, S. Manley, J. C. Ye, and M. Unser, "FALCON: fast and unbiased reconstruction of high-density super-resolution microscopy data," *Scientific Reports*, vol. 4, no. 1, p. 4577, 2015.

[8] D. Sage, H. Kirshner, T. Pengo, N. Stuurman, J. Min, S. Manley, and M. Unser, "Quantitative evaluation of software packages for single-molecule localization microscopy," *Nature Methods*, vol. 12, no. 8, pp. 717–724, 2015.

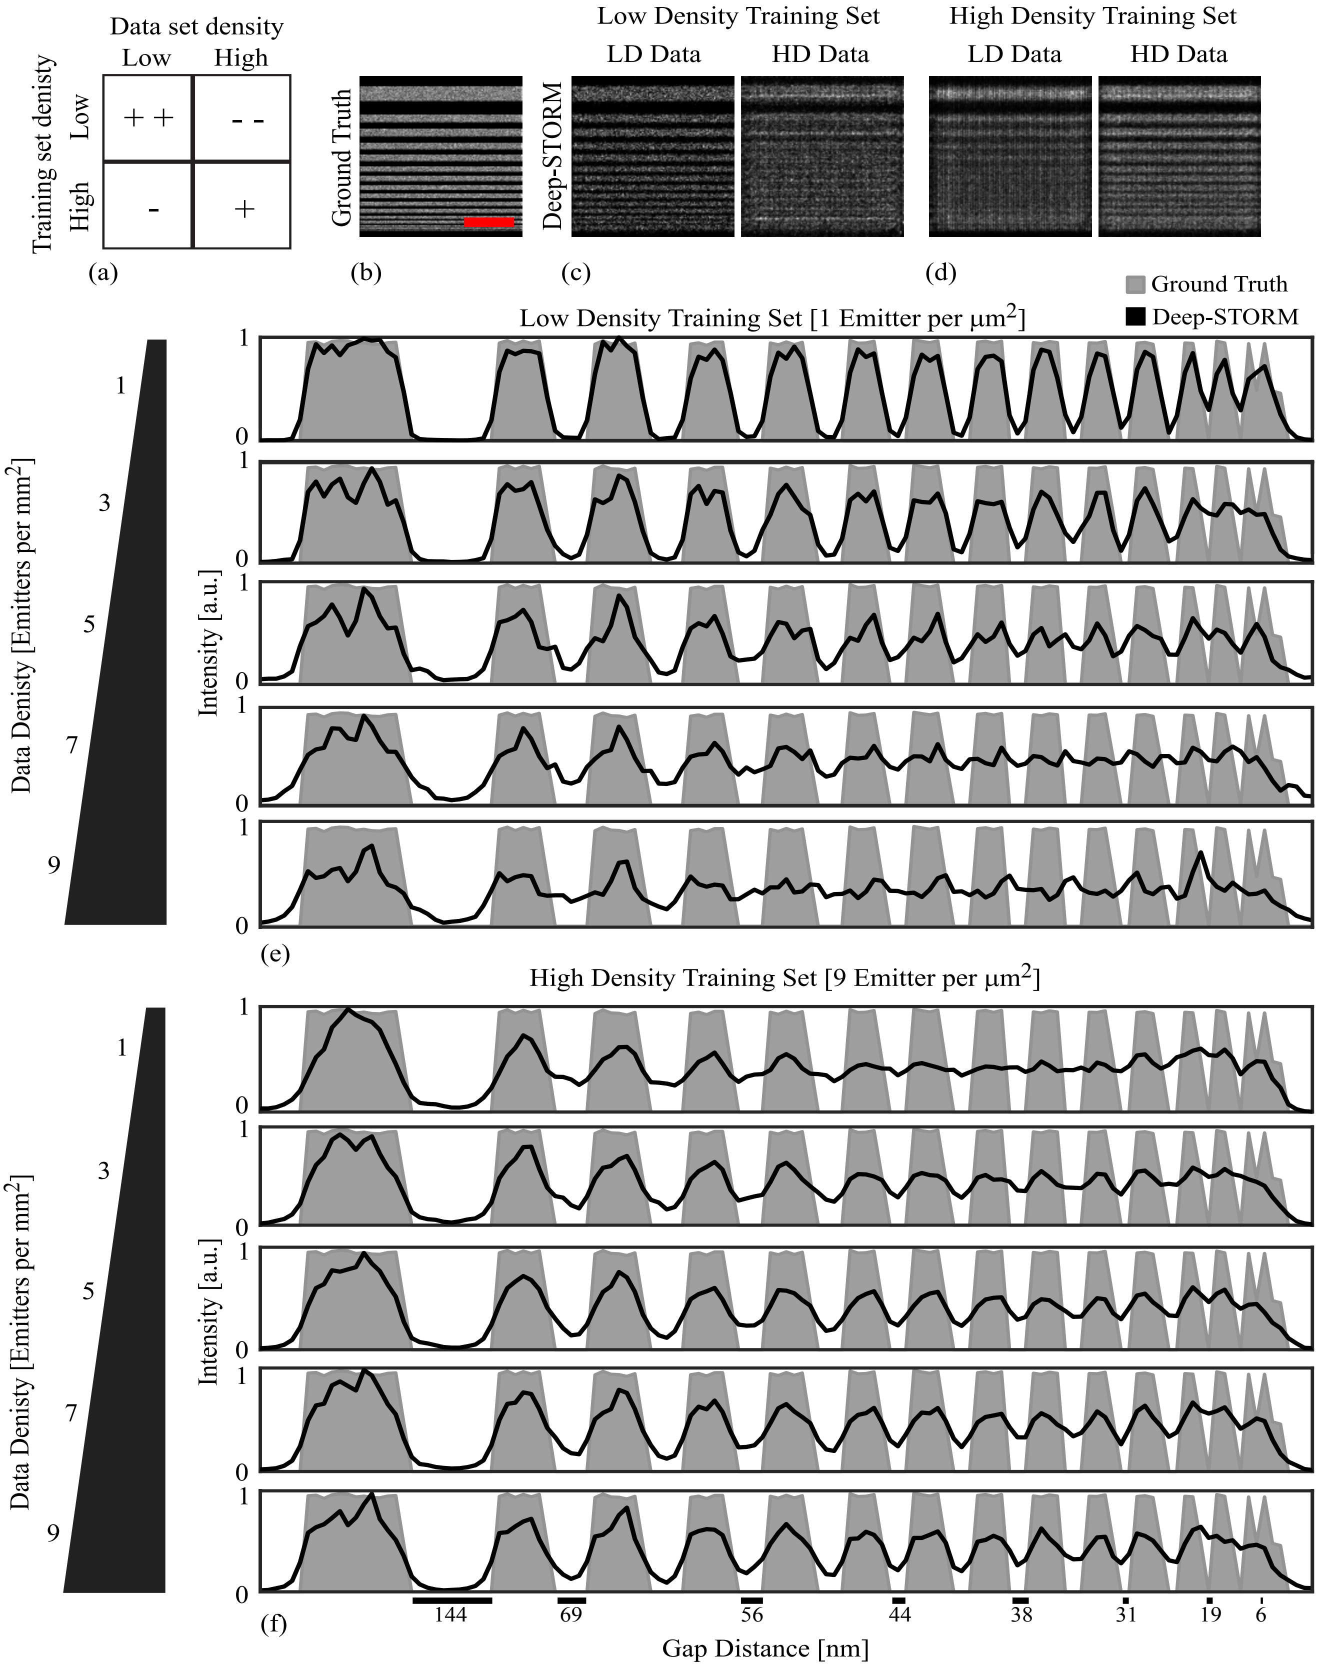


**Fig. 8.** Evaluation of resolution as a function of emitter density. (a) Deep-STORM exhibits the best performance when trained on a dataset with similar density to the evaluation data. (b) Emitters were simulated on horizontal lines with decreasing widths and gaps. Scalebar 500 nm. (c) Deep-STORM was evaluated on low density (LD) and high density (HD) data with a low-density training set. (d) Deep-STORM using a high-density training set. (e) The projection of the ground truth (gray) and LD-trained Deep-STORM reconstruction (black lines) with 5 densities. (f) Same as d, but with Deep-STORM trained on an HD dataset.

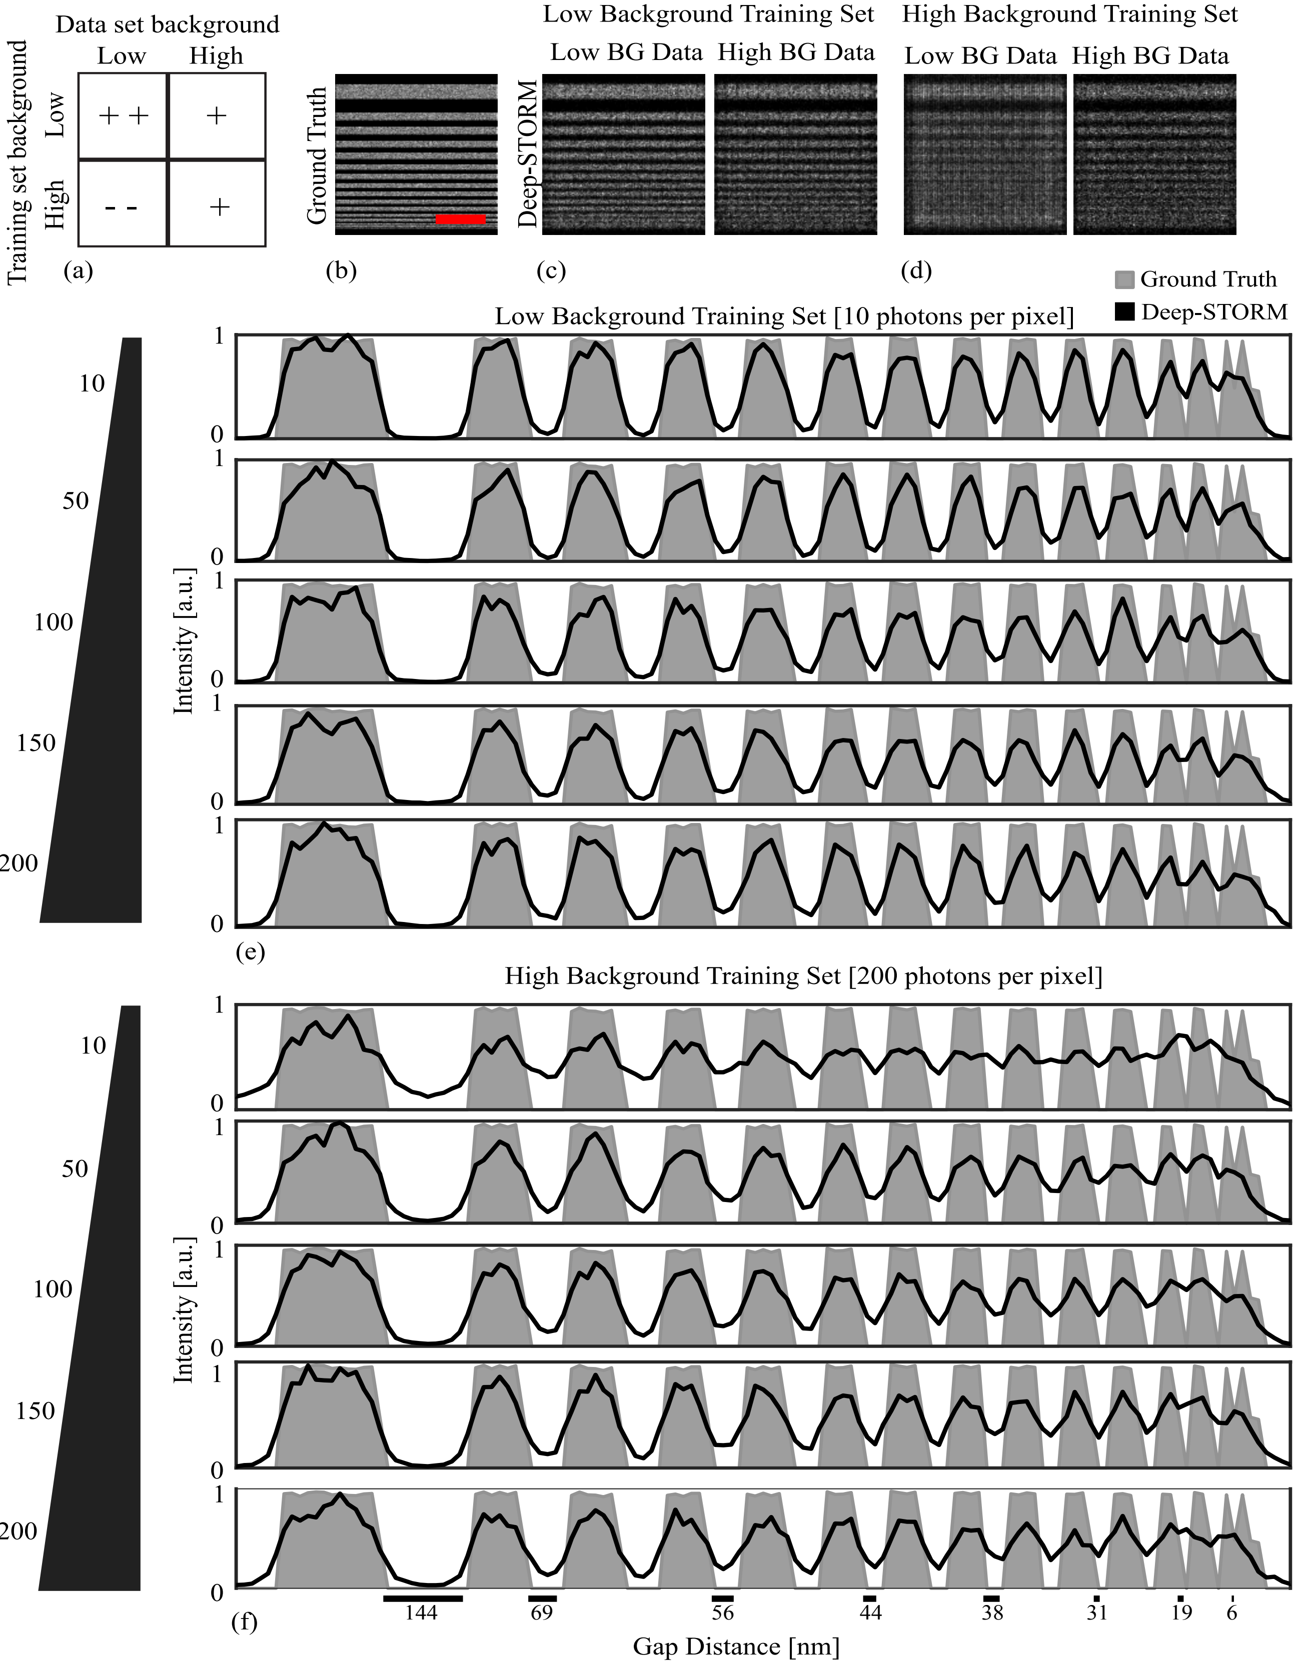


**Fig. 9.** Evaluation of resolution as a function of the signal-to-noise ratio. (a) Deep-STORM exhibits the best performance when trained on a dataset with similar density to the evaluation data, but is also robust to higher backgrounds than the training data set. (b) Emitters were simulated on horizontal lines with decreasing widths and gaps. Scalebar 500 nm. (c) Deep-STORM was evaluated on low background (BG) and high BG data with a low BG training set. (d) Deep-STORM using a high-BG training set. (e) The projection of the ground truth (gray) and low-BG-trained Deep-STORM reconstruction (black lines) with 5 background levels. (f) Same as d, but with Deep-STORM trained on a high-background dataset.
